# Supplementary material for: Higher Order Topological Phases: A General Principle of Construction
Source: arXiv:1808.08965 ancillary file (2019-02-13)
Supplement: Supplementary file 1 [file Supplementary.pdf]

# Supplementary Materials for "Higher Order Topological Phases: A General Principle of Construction"


Dumitru Călugăru,[1,2] Vladimir Juričić,[3] and Bitan Roy[1]

[1]Max-Planck-Institut für Physik komplexer Systeme, Nöthnitzer Stra. 38, 01187 Dresden, Germany
[2]Cavendish Laboratory, University of Cambridge,
J. J. Thomson Avenue, Cambridge, CB3 0HE, United Kingdom
[3]Nordita, KTH Royal Institute of Technology and Stockholm University, Roslagstullsbacken 23, 10691 Stockholm, Sweden


This Supplementary Material contains:


**I. Numerical Methods for Constructing the Topological Surface States**

**II. Second-order Topological Insulator**

**III. Higher order Nodal-loop semimetal**

**IV. Higher Order Topological Dirac Semimetals**
IV.A. Double-component ($s = 1/2$) TDSM
IV.B. Triple-component ($s = 1$) TDSM
IV.C. Generalization of the matrix $M$ for an arbitrary spin $s$

**References**


## I. NUMERICAL METHODS FOR CONSTRUCTING THE TOPOLOGICAL SURFACE STATES

This section aims to present and discuss the general numerical approach that was used to extract the surface states for the different topological semimetals discussed in the main paper. Our analysis is based on lattice tight-binding models, which take the following general form:

$$H = \sum_{\mathbf{k}} \Psi^{\dagger}(\mathbf{k}) \left[ \sum_i N_i(\mathbf{k}) \Gamma_i + \sum_j \Delta_j N'_j(\mathbf{k}) \Gamma'_j \right] \Psi(\mathbf{k}). \tag{1}$$

In Eq. (1), $\Gamma_i$ and $\Gamma'_j$ represent $n$-dimensional Hermitian matrices and $\Psi(\mathbf{k})$ is an $n$-component annihilation operator. The first term in the Hamiltonian refers to the unperturbed semimetal to which appropriate perturbations are added for the realization of higher-order topological semimetals. This construction can be generalized, however, for the realization of higher-order topological insulators (discussed in Sec. II). The matrices in the perturbation term ($\Gamma'_i$) are chosen in accordance to the following anticommutation algebra:

$$\left\{ \Gamma'_i, \Gamma'_j \right\} = 2\, \delta_{ij}\, I, \quad \left\{ \Gamma_i, \Gamma'_j \right\} = 0, \tag{2}$$

where $\delta_{ij}$ is the Kronecker $\delta$ symbol. Therefore, as discussed in the main paper, the zero-energy surface modes can be selectively gapped according to the form factors $N'_j(\mathbf{k})$. These are chosen to vanish at the band-touching points preserving the topological semimetal character.

Typically, we consider a simple cubic lattice (of lattice constant $a$) with open boundary conditions (OBC). Alternatively, to better understand the origin of the surface states, mixed boundary conditions (MBC) are employed, imposing OBC in the directions perpendicular to the surfaces of interest, while keeping periodic boundary conditions (PBC) in the other directions. For this purpose, we employ either a Wannier or a mixed Wannier-Bloch representation, both of which can be generically written as

$$\Psi_\alpha(\mathbf{k}) = \frac{1}{\sqrt{L^p}} \sum_{x_{j_1}, x_{j_2}, \ldots} \exp(i k_{j_1} a x_{j_1} + i k_{j_2} a x_{j_2} + \ldots) \Psi_\alpha\left(k_{i_1}, k_{i_2}, \ldots; x_{j_1}, x_{j_2}, \ldots\right), \tag{3}$$

where $L$ represents the system size along the $p$ directions in which OBC are imposed. We label the indices of the lattice sites in the $j$ direction with $x_j \in \mathbb{Z}$ and $\alpha$ labels the components of the annihilation operator. In this basis,

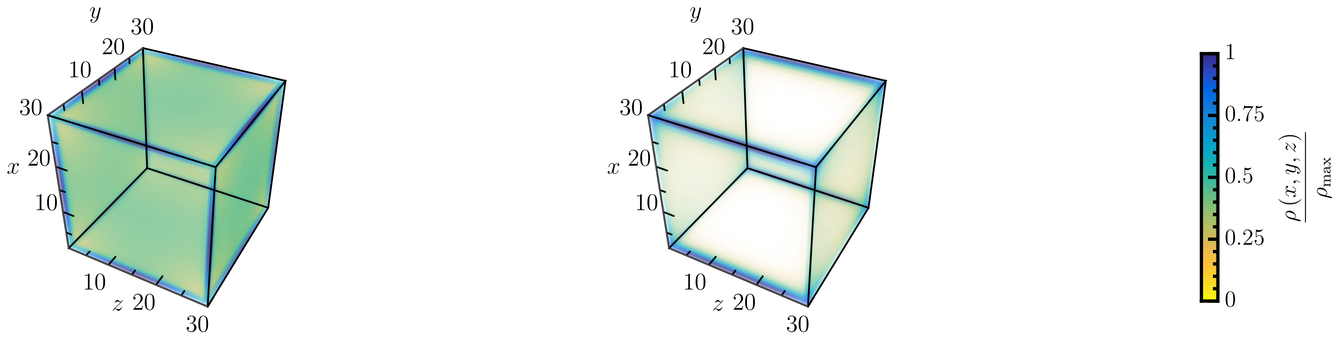


(a) (b)

FIG. S1: The surface states of a 1st-order (a) and a 2nd-order (b) topological insulator. We plot the square of the amplitude of the state with the smallest absolute energy ($E = \mathcal{O}(10^{-2})$), $\rho(x, y, z)$, which is normalized to lie in the interval $[0, 1]$. The system size is $L = 30$, and $\Delta_1 = 0.3$ for panel (b).

the Hamiltonian is given by

$$H = \sum_{\substack{x_{j_1}, x_{j_2}, \dots \\ x'_{j_1}, x'_{j_2}, \dots \\ k_{i_1}, k_{i_2}, \dots \\ \alpha, \beta}} \Psi^\dagger_\alpha \left(k_{i_1}, k_{i_2}, \dots; x'_{j_1}, x'_{j_2}, \dots\right) h^{\alpha\beta} \left(k_{i_1}, k_{i_2}, \dots; x_{j_1}, x'_{j_1}, x_{j_2}, x'_{j_2}, \dots\right) \Psi_\beta \left(k_{i_1}, k_{i_2}, \dots; x_{j_1}, x_{j_2}, \dots\right). \tag{4}$$

The matrix $h$ is obtained by Fourier transforming the Hamiltonian in Eq. (1)

$$\begin{aligned} &h^{\alpha\beta}\left(k_{i_1}, k_{i_2}, \dots; x_{j_1}, x'_{j_1}, x_{j_2}, x'_{j_2}, \dots\right) = \\ &= \frac{1}{L^p} \sum_{k_{j_1}, k_{j_2}, \dots} \left[ \sum_i N_i(\mathbf{k}) \Gamma^{\alpha\beta}_i + \sum_j \Delta_j N'_j(\mathbf{k}) \Gamma'^{\alpha\beta}_j \right] \exp[i k_{j_1} a (x_{j_1} - x'_{j_1}) + i k_{j_2} a (x_{j_2} - x'_{j_2}) + \dots]. \end{aligned} \tag{5}$$

The advantage of using this representation when MBC are employed is that $h$ is block-diagonal in the momenta $k_i$ (corresponding to the directions along which PBC were imposed and translational symmetry is preserved). For the numerical implementation, we consider a finite system along the open-boundary directions, with $L^p$ lattice sites and take

$$h^{\alpha\beta}\left(k_{i_1}, k_{i_2}, \dots; x_{j_1}, x'_{j_1}, x_{j_2}, x'_{j_2}, \dots\right) = 0, \tag{6}$$

for any $x_i, x'_i > L$ or $x_i, x'_i < 1$.

Since the semimetals we consider exhibit particle-hole symmetry, we isolate the surface states by effectively selecting those eigenstates with $|E| < \epsilon$ (where $\epsilon$ is a small number). In constructing the solutions $\Psi_\beta(x, y, z)$ for the surface states, we numerically diagonalized the $nL^3 \times nL^3$ Hamiltonian matrix $h^{\alpha\beta}(x, x', y, y', z, z')$. Alternatively, when MBC are imposed, the solution $\Psi_\beta(k_{i_1}, k_{i_2}, \dots; x_{j_1}, x_{j_2}, \dots)$ for the surface state is determined by diagonalizing the $nL^p \times nL^p$ Hamiltonian matrix $h^{\alpha\beta}\left(k_{i_1}, k_{i_2}, \dots; x_{j_1}, x'_{j_1}, x_{j_2}, x'_{j_2}, \dots\right)$ for different values of $k_i$. For each point in the momentum space $(k_{i_1}, k_{i_2}, \dots)$, we determined the eigenvector with the minimum absolute energy. The obtained value of $E(k_{i_1}, k_{i_2}, \dots)$ was compared with 0 within a tolerance $\epsilon$. In the cases where $|E(k_{i_1}, k_{i_2}, \dots)| < \epsilon$, the respective eigenvector was used to construct $\Psi_\beta(k_{i_1}, k_{i_2}, \dots; x_{j_1}, x_{j_2}, \dots)$ for the point $(k_{i_1}, k_{i_2}, \dots)$ in momentum space. Otherwise, $\Psi_\beta(k_{i_1}, k_{i_2}, \dots; x_{j_1}, x_{j_2}, \dots)$ was assigned 0 for all the values of $(x_{j_1}, x_{j_2}, \dots)$. This allows the visualization of surface states in mixed real-space-momentum representation.

Additionally, in the case of systems with flat, non-dispersive bands at $E = 0$, we select the surface states based on their degree of boundary localization in addition to their energy (see Sec. IV.B).

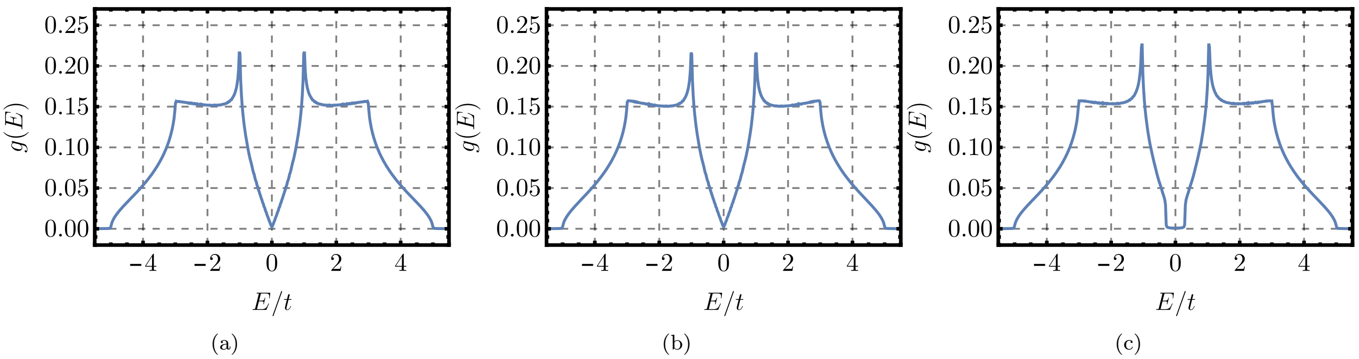


FIG. S2: The effects of momentum dependent perturbations on the density of states in the case of a 1st-order (a) and 2nd-order (b) nodal-loop semimetal compared to a constant perturbation (c). Because the functions $N_i'$ vanish at the band-touching points, they preserve the form of the density of states of the system near $E = 0$, namely $g(E) \sim |E|$. On the other hand, suppressing the momentum dependence of $N_i'$ (i.e. setting $N_i' = 1$) produces a hard gap and the system becomes an insulator.

## II. SECOND-ORDER TOPOLOGICAL INSULATOR

We start by implementing a topological insulator[1] (TI) with

$$\begin{aligned} &N_1(\mathbf{k}) = M + t[\cos(k_x a) + \cos(k_y a) + \cos(k_z a)],\ N_1'(\mathbf{k}) = \cos(k_x a) - \cos(k_y a), \\ &N_2(\mathbf{k}) = \eta \sin(k_x a), N_3(\mathbf{k}) = \eta \sin(k_y a), N_4(\mathbf{k}) = \eta \sin(k_z a). \end{aligned} \tag{7}$$

We choose $t = \eta = 1$ and $M = -2$ for the numerical implementation, such that for $\Delta_1 = 0$, the system represents a strong TI. A four-band model is constructed by choosing $\Gamma_1 = \tau_3 \otimes \sigma_0$, $\Gamma_{i+1} = \tau_1 \otimes \sigma_i$ (for $i = 1, 2, 3$) and $\Gamma_1' = \tau_2 \otimes \sigma_0$. $\{\sigma_\mu\}$ and $\{\tau_\mu\}$ represent two-dimensional Pauli matrices which, respectively, operate on the spin and orbital indices.

The surface states in a 1st-order ($\Delta_1 = 0$) and a 2nd-order ($\Delta_1 \neq 0$) TI are visualized by employing OBC in all directions and plotting the amplitude lowest energy state (i.e. the state $i$ for which $|E_i|$ is minimal) given by

$$\rho(x, y, z) = \left\langle \Psi_i^\dagger(x, y, z) \Psi_i(x, y, z) \right\rangle . \tag{8}$$

A 1st-order TI displays surface states which cover all the faces of a cubic crystal, while the presence of the perturbation promotes the formation of hinge states parallel to the $\hat{\mathbf{z}}$ direction in a 2nd-order TI.

## III. HIGHER ORDER NODAL-LOOP SEMIMETAL

The particular form of the nodal-loop semimetal (NLSM) we consider in the main text reads

$$\begin{aligned} &N_1(\mathbf{k}) = t[\cos(k_x a) + \cos(k_y a) - b] + tN''(\mathbf{k}),\ N_2(\mathbf{k}) = t\sin(k_z a),\ N_1'(\mathbf{k}) = N''(\mathbf{k}) \sin(k_x a) \sin(k_y a), \\ &N_2'(\mathbf{k}) = N''(\mathbf{k})[\cos(k_x a) - \cos(k_y a)],\ N_3'(\mathbf{k}) = N''(\mathbf{k})[\cos(k_x a) + \cos(k_y a) - b'], \end{aligned} \tag{9}$$

where $N''(\mathbf{k}) = \cos(k_z a) - 1$. This topological semimetal presents a nodal loop in the $k_z = 0$ plane, where the functions multiplying the $\Gamma_i'$ matrices vanish. In our computations, we set $a = 1$, $t = 1$, $b = 1$ and $b' = 1.5$.

As far as the choice of matrices is concerned, two cases could be considered. Neglecting the spin of the fermion, we can choose $\Gamma_1 = \sigma_1$, $\Gamma_2 = \sigma_2$ and $\Gamma_i' = \sigma_3$. The lack of a fourth matrix in the space of mutually anticommuting two-dimensional Hermitian matrices results in no more than one perturbation which can be introduced, implying that at most a second-order NLSM could be realized. We focus on the case when the spin degree of freedom is taken into account and construct a four-band model by choosing $\Gamma_1 = \sigma_0 \otimes \tau_1$, $\Gamma_2 = \sigma_0 \otimes \tau_2$ and three distinct matrices $\Gamma_i' = \sigma_i \otimes \tau_3$ satisfying Eq. (2). In what follows, we set $\Delta_i = 0.3$, for all $i \leq n$ for the realization of a $(n+1)^{\text{th}}$-order NLSM, leaving $\Delta_j = 0$ for $j > n$.

To show that these perturbations do not affect the bulk topology of the semimetal, one can consider the effects they have on the density of states (DoS), particularly in the vicinity of the band touching points (Fig. S2). The DoS, $g(E)$, does not change significantly, maintaining the same power-law dependence, $g(E) \sim |E|$, as opposed to the

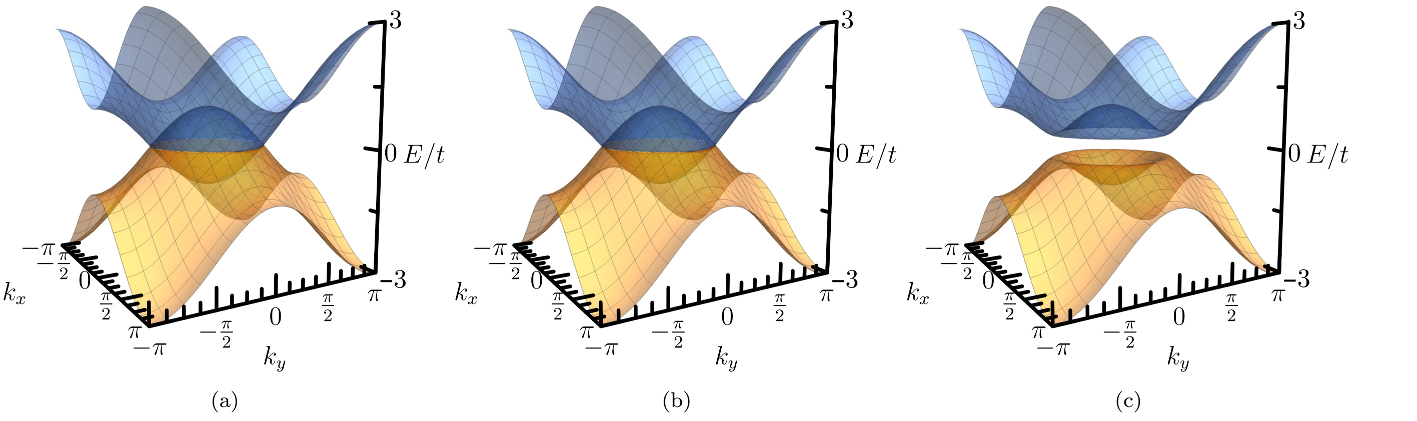


FIG. S3: The effects of momentum dependent perturbations on the band structure in the $k_z = 0$ plane for the case of a $1^{\text{st}}$-order (a) and $2^{\text{nd}}$-order (b) nodal-loop semimetal compared to a constant perturbation (c). The band touching points are not affected by the presence of the perturbation $\Delta_1 = 0.3$. A constant perturbation ($N_i' = 1$) however, produces a hard gap and the system becomes insulating. Although not shown explicitly, the same conclusion holds for the $3^{\text{rd}}$-order and $4^{\text{th}}$-order nodal-loop semimetals.

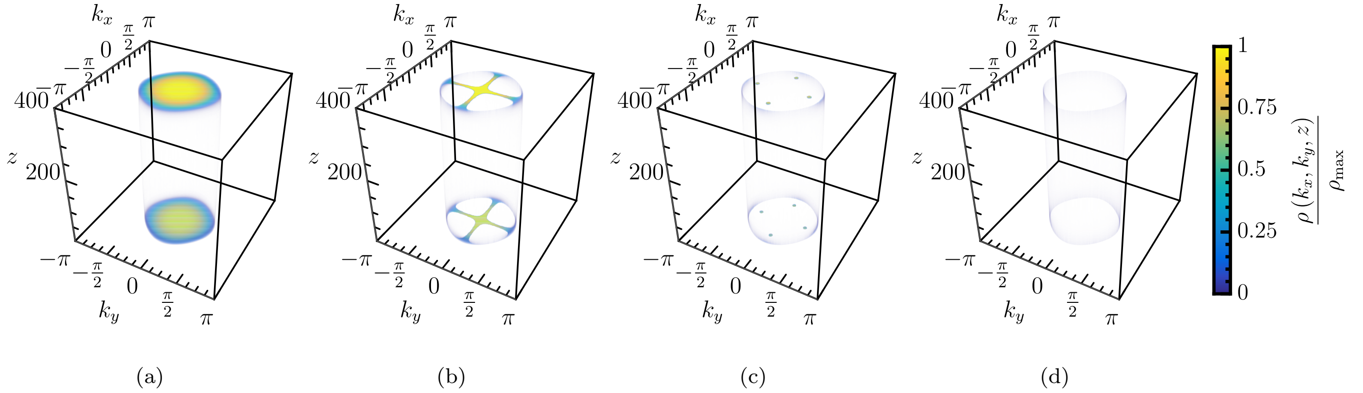


FIG. S4: The surface states of a $1^{\text{st}}$-order (a), $2^{\text{nd}}$-order (b), $3^{\text{rd}}$-order (c) and $4^{\text{th}}$-order (d) nodal-loop semimetal shown in a mixed momentum-real space representation. There is an effective dimensionality reduction in the momentum space corresponding to an increase in the order of the nodal-loop semimetal. The lattice size along the $\hat{\mathbf{z}}$ direction is $L = 400$. In all cases, we set $\epsilon = 0.01$ to improve the readability of the plots, but the surface states themselves have energies $E = \mathcal{O}\left(10^{-15}\right)$.

case where constant perturbations are introduced and a hard band gap forms. This is further supported by the band structure in the $k_z = 0$ plane (Fig. S3).

To compute the local density of states (LDoS) we use

$$\rho(x,y,z) = \sum_{\substack{i \\ |E_i|<\epsilon}} \left\langle \Psi_i^\dagger(x,y,z)\Psi_i(x,y,z)\right\rangle . \tag{10}$$

employing OBC, which yields Fig. 3 of the main paper.

Setting $\epsilon = 0.003$, we find that the LDoS is formed by summing over 348 and over 20 states for a $1^{\text{st}}$-order and a $2^{\text{nd}}$-order NLSM, respectively. As there are only four equivalent states in the momentum space for a $3^{\text{rd}}$-order NLSM, we plot only the amplitude lowest lying surface state (i.e. $|E_i|$ is minimal) according to Eq. (8) .

By imposing OBC only along the $\hat{\mathbf{z}}$ direction, the resulting surface states are presented in Fig. S4. After finding the solution in the Wannier-Bloch representation corresponding to the surface states ($\Psi\left(k_x,k_y,z\right)$), we calculate their squared amplitude

$$\rho\left(k_x,k_y,z\right) = \left\langle \Psi^\dagger\left(k_x,k_y,z\right)\Psi\left(k_x,k_y,z\right)\right\rangle . \tag{11}$$

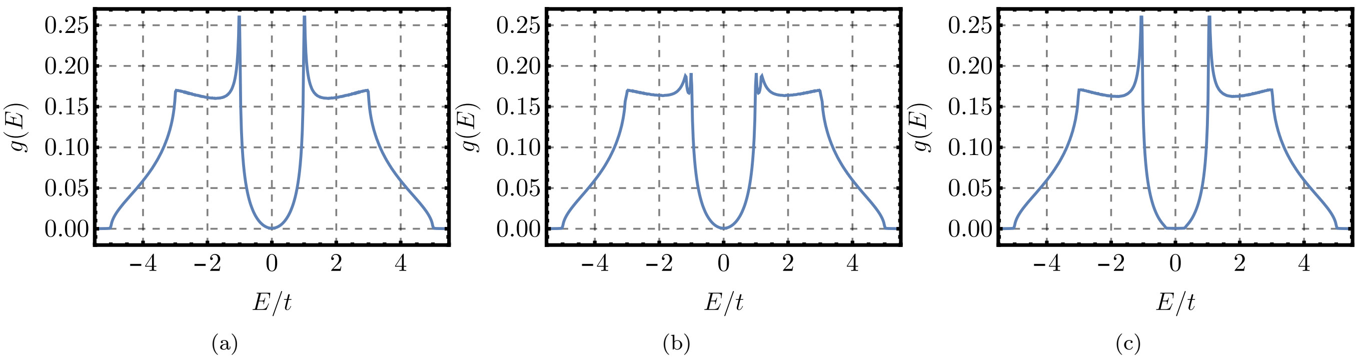


FIG. S5: The effects of momentum dependent perturbations on the density of states in the case of a $1^{\mathrm{st}}$-order (a) and $2^{\mathrm{nd}}$-order (b) spin-1/2 Dirac semimetal compared to a constant perturbation (c). The quadratic shape of the density of states near $E = 0$ is protected by appropriately choosing the functions $N_i'$. In contrast, constant perturbations introduce a hard band gap.

In the unperturbed case, the surface states form a filled circle corresponding exactly to the nodal loop that merges with the bulk states at the perimeter. As different perturbations are introduced, the surface states are restricted to the locus of points in the $(k_x, k_y)$ plane where the functions $N_i'(\mathbf{k})$ vanish. For the case of a $2^{\mathrm{nd}}$-order NLSM, the remaining surface states are arranged in the shape of a cross, while for a $3^{\mathrm{rd}}$-order NLSM they consist of only four points in the momentum space. No surface localized state is present in the case of a $4^{\mathrm{th}}$-order NLSM.

## IV. HIGHER ORDER TOPOLOGICAL DIRAC SEMIMETALS

Next, we turn our focus to topological Dirac semimetals (TDSMs) realized by taking

$$\begin{aligned} &N_1(\mathbf{k}) = t\sin(k_x a),\ N_2(\mathbf{k}) = t\sin(k_y a),\ N_3(\mathbf{k}) = t[\cos(k_x a) + \cos(k_y a) - 2] + t\cos(k_z a), \\ &N_1'(\mathbf{k}) = \cos(k_x a) - \cos(k_y a),\ N_2'(\mathbf{k}) = \sin(k_x a)\sin(k_y a)\sin(k_z a). \end{aligned} \tag{12}$$

The functions $N_i'$ are chosen to protect the Dirac points located at $\mathbf{k} = (0, 0, \pm\pi/2)$. The form of the perturbations will at most alter the Fermi velocity at the band touching points, but will not gap the system. The choice of the matrices depends on the particular type of system we want to study. We consider two cases: a (pseudo-)spin-1/2 (double-component) and a (pseudo-)spin-1 (triple-component) TDSM.

### IV.A. Double-component ($s = 1/2$) TDSM

In the $s = 1/2$ case, we choose the five anticommuting $4\times4$ matrices to be: $\Gamma_1 = \tau_3\otimes\sigma_1$, $\Gamma_2 = \tau_0\otimes\sigma_2$, $\Gamma_3 = \tau_0\otimes\sigma_3$, $\Gamma_1' = \tau_1\otimes\sigma_1$ and $\Gamma_2' = \tau_2\otimes\sigma_1$. We check again that introducing the various Wilson masses does not change the DoS near the band touching point (Fig. S5) or the band structure (Fig. S6).

In what follows, we set $\Delta_i = 0.3$, for all $i \le n$ for the realization of a $(n+1)^{\mathrm{th}}$-order TDSM, and $\Delta_j = 0$ for $j > n$. We furthermore employ OBC along the $\hat{\mathbf{x}}$ and $\hat{\mathbf{y}}$ directions for the visualization of the surface states (Fig. S7). The Fermi arc state stretches between the two Dirac points, merging with the delocalized bulk states at the band touching points and covering the whole surfaces tangential to $\hat{\mathbf{z}}$. The surface states become hinge states in a $2^{\mathrm{nd}}$-order TDSM, and are reduced to just one state in a $3^{\mathrm{rd}}$-order TDSM. The presence of the delocalized zero-energy bulk states at the Dirac points confirms the semimetalic character of the higher-order TDSMs.

### IV.B. Triple-component ($s = 1$) TDSM

The case of a triple Dirac semimetal can be thought of as a generalization of the previous case. Such a generalization requires that we choose $\Gamma_1 = \tau_3\otimes S_1$, $\Gamma_2 = \tau_0\otimes S_2$ and $\Gamma_3 = \tau_0\otimes S_3$, where $S_i$ represent the spin-1 matrices. Note that although the $\Gamma_i$ matrices do not follow the same commutation algebra of the $S_i$ matrices, the introduction of direct products merely doubles the degeneracy of each level, but does not change the energy spectrum. For the

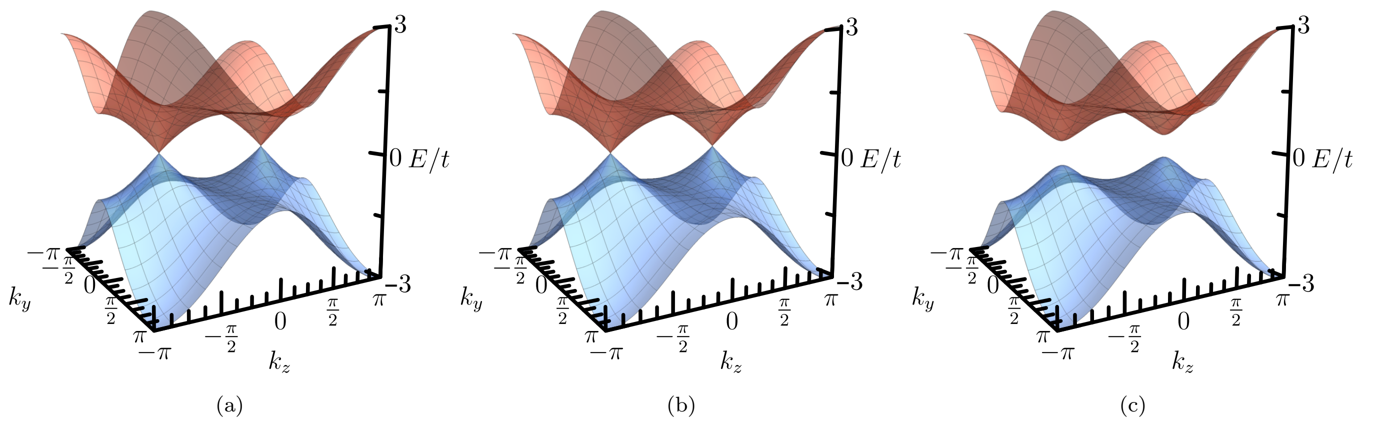


FIG. S6: The effects of momentum dependent perturbations on band structure in the $k_x = 0$ plane in the case of a 1$^{\text{st}}$-order (a) and 2$^{\text{nd}}$-order (b) spin-1/2 Dirac semimetal compared to a constant perturbation (c). Each band is doubly degenerate. The perturbations do not affect the band structure. Suppressing the momentum dependence of $N_i'$ produces a hard gap and the system becomes an insulator.

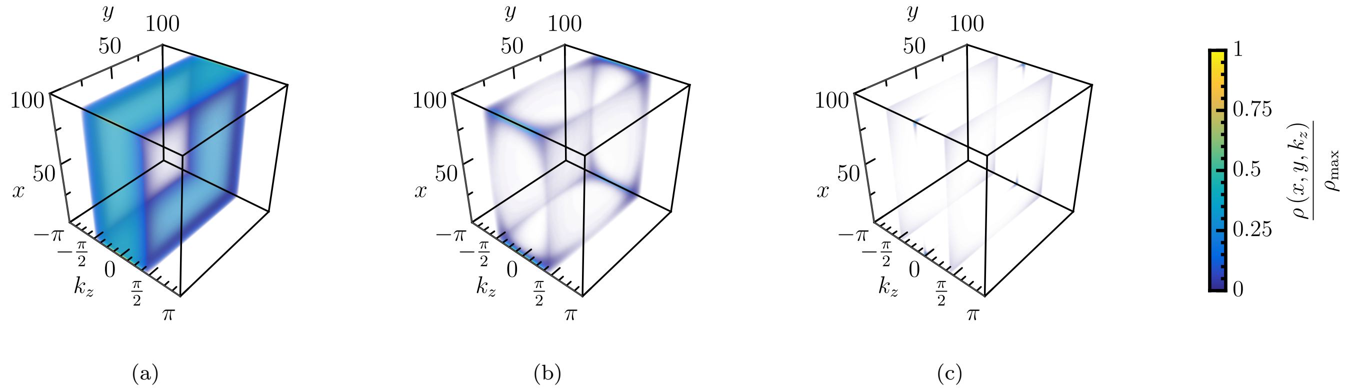


FIG. S7: The surface states in a 1$^{\text{st}}$-order (a), 2$^{\text{nd}}$-order (b) and 3$^{\text{rd}}$-order (c) spin-1/2 Dirac semimetal. The maximum value of the density $\rho_{\max}$ is not the same across the different figures in order to improve readability. The energy limit $\epsilon$ for each case was chosen to be, respectively: 0.01, 0.01 and 0.001. In all cases, we set the lattice size along the $\hat{\mathbf{x}}$ and $\hat{\mathbf{y}}$ direction is $L = 100$.

perturbations, the matrices $\Gamma_i'$ need to anticommute with each other, and also with all the $\Gamma_i$ matrices. The solution is $\Gamma_i' = \tau_i \otimes M$ with $i = 1, 2$, where the matrix $M$ satisfies $[M, S_1] = \{M, S_2\} = \{M, S_3\} = 0$, yielding

$$M = \begin{bmatrix} 0 & 0 & 1 \\ 0 & 1 & 0 \\ 1 & 0 & 0 \end{bmatrix}. \tag{13}$$

A generalization of this approach for an arbitrary spin $s$ is presented in subsection IV.C.

Since the functions $N_i'(\mathbf{k})$ vanish at the Dirac points, the semimetalic character of the higher-order systems is preserved. An inspection of the band structure (Fig. S8) reveals that the topologically non-trivial bands are not affected by the introduction of these Wilson masses near the triple points.

Similar to the $s = 1/2$ case, we employ OBC in all directions in order to visualize the surface states in real space. A complication arises in this system due to the presence of two flat, dispersionless bands at precisely $E = 0$. This means that the degree of boundary localization, $\rho_i^{\partial S}$, has to be considered for the determination of surface states, in

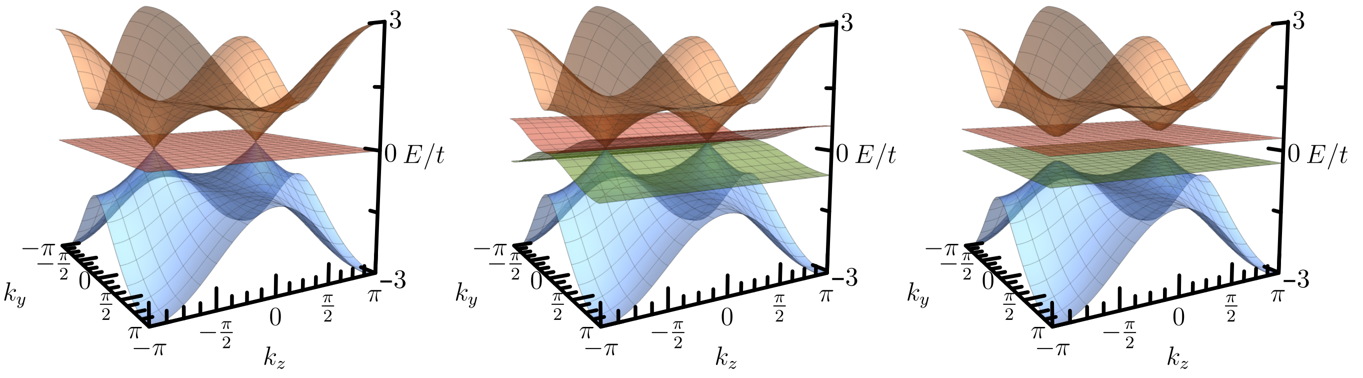


FIG. S8: Same as in Fig. S6, but for a spin-1 Dirac semimetal. The figures show that the topologically non-trivial bands in (a) are not affected by the introduction of various Wilson masses near the triple points ($\Delta_1 = 0.3$). Suppressing the momentum dependence of the perturbations in (c) produces a hard gap and the system becomes insulating.

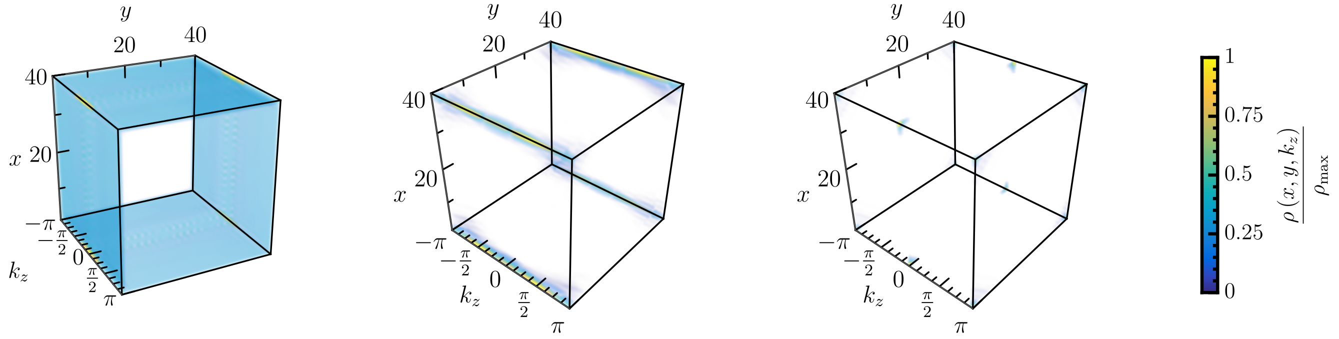


FIG. S9: Same as in Fig. S7, but for a spin-1 Dirac semimetal. The number of lattice points along the $\hat{\mathbf{x}}$ and $\hat{\mathbf{y}}$ directions is $L = 40$. We set the energy limit $\epsilon$ to be 0.04, 0.04 and 0.02, respectively, for the three cases.

addition to the energies $E_i$. Depending on the type of perturbation introduced, $\rho_i^{\partial S}$ is defined as

$$\rho_i^{\partial S} = \begin{cases} \sum\limits_{\substack{1\leq x,y,z\leq L \\ \{1,L\}\cap\{x,y,z\}\neq\emptyset}} \rho_i(x,y,z) & \Delta_2 = 0 \\ \sum\limits_{x,y,z\in\{1,L\}} \rho_i(x,y,z) & \Delta_2 \neq 0, \end{cases} \tag{14}$$

where $\rho_i(x,y,z) = \left\langle \Psi_i^\dagger(x,y,z)\,\Psi_i(x,y,z)\right\rangle$. These two expressions for the degree of boundary localization correspond to the probability density on the surface and on the corners of the crystal, respectively. In Fig. 2 of the main paper, we select the maximally localized states (i.e. the states with the highest value of $\rho_i^{\partial S}$) that have $|E_i| < \epsilon$ (with $\epsilon = 0.05$). These states have $|E| = \mathcal{O}\left(10^{-7} - 10^{-2}\right)$.

We also employ the degree of boundary localization, $\rho_i^{\partial S}(k_z)$, when considering OBC only in the $\hat{\mathbf{x}}$ and $\hat{\mathbf{y}}$ directions (Fig. S9), in addition to the energies $E_i(k_z)$. Depending on the type of perturbation considered, $\rho_i^{\partial S}(k_z)$ is defined as

$$\rho_i^{\partial S}(k_z) = \begin{cases} \sum\limits_{\substack{1\leq x,y\leq L \\ \{1,L\}\cap\{x,y\}\neq\emptyset}} \rho_i(x,y,k_z) & \Delta_1 = 0 \\ \rho_i(1,1,k_z) + \rho_i(L,1,k_z) + \rho_i(1,L,k_z) + \rho_i(L,L,k_z) & \Delta_1 \neq 0, \end{cases} \tag{15}$$

for each value of $k_z$. The restriction to just the corners of the lattice reflects the effect of the first perturbation

to produce hinge states (in the mixed real-space-momentum representation). In constructing the full surface state, for each value of $k_z$, we choose the states with the highest degree of boundary localization that additionally satisfy $|E_i(k_z)| < \epsilon$.

In order to form an $(n+1)^{\text{th}}$-order triple-component TDSM, we set $(\Delta_1, \Delta_2) = (0.1, 0)$ for a $2^{\text{nd}}$-order and $(\Delta_1, \Delta_2) = (0.1, 0.2)$ for a $3^{\text{rd}}$-order triple-component TDSM. A $1^{\text{st}}$-order spin-1 TDSM has two surface arc states linking the triple points in opposite directions along the $\hat{\mathbf{z}}$ direction in momentum space. The result is a surface state that stretches along the complete range $k_z \in [-\pi/a, \pi/a]$. The Wilson masses act in a similar fashion to the spin-1/2 case. Namely, edge states are introduced in a $2^{\text{nd}}$-order triple TDSM for all values of the momenta $k_z$ (yielding hinge modes in the real space), while in a $3^{\text{rd}}$-order triple TDSM, the additional Wilson mass selectively gaps all but the edge states at $k_z = 0, \pi/a$, ultimately producing corner states in the real space (Fig. 2 of the main paper).

### IV.C. Generalization of the matrix $M$ for an arbitrary spin $s$

In this section we illustrate how the scheme of generating higher order topological phases can be generalized to TDSMs belonging to an arbitrary spin-$s$ representation. For this purpose, the same construction as the one in subsection IV.B can be applied by replacing the spin-1 matrices with spin-$s$ matrices. Similarly, the new operator $M$ must obey

$$[M, S_1] = 0,\ \{M, S_2\} = 0,\ \{M, S_3\} = 0, \tag{16}$$

with $S_i$ being $(2s+1)$-dimensional spin-$s$ matrices (where $s$ can be integer or half-integer). The first two of these relations can be written more succinctly using the ladder operators ($S_\pm = S_1 \pm iS_2$) as

$$MS_+ = S_- M. \tag{17}$$

Intuitively, we can infer the effect of $M$ from the Eq. (17) and the last relation of Eq. (16): $M$ simply reflects the spin eigenstates in the $xy$ plane. Working in the canonical eigenbasis of $S_3$, $|s, m\rangle$, we can prove that the operator

$$M = \sum_{m,s} |s, m\rangle \langle s, -m| \tag{18}$$

obeys the necessary algebra. First let us verify that it satisfies $\{M, S_3\} = 0$:

$$MS_3 = \sum_{m,s} |s, m\rangle \langle s, -m| S_3 = \sum_{m,s} -m |s, m\rangle \langle s, -m| = \sum_{m,s} -S_3 |s, m\rangle \langle s, -m| = -S_3 M. \tag{19}$$

Similarly, we can show that Eq. (17) is satisfied

$$\begin{aligned} MS_+ &= \sum_{\substack{m,s \\ m',s'}} |s, m\rangle \langle s, -m| \sqrt{s'(s'+1) - m'(m'+1)}\, |s', m'+1\rangle \langle s', m'| = \\ &= \sum_{\substack{m,s \\ m',s'}} \delta_{s,s'} \delta_{-m,m'+1} \sqrt{s'(s'+1) - m'(m'+1)}\, |s, m\rangle \langle s', m'| = \\ &= \sum_{m,s} \sqrt{s(s+1) - m(m+1)}\, |s, -m-1\rangle \langle s, m| = \\ &= \sum_{m,s} S_- |s, -m\rangle \langle s, m| = \\ &= S_- M. \end{aligned} \tag{20}$$

Thus, higher order topological phases can be realized using a similar approach to the one presented in the main paper for a TDSM with an arbitrary (pseudo)-spin $s$.

[1] F. Schindler, A. M. Cook, M. G. Vergniory, Z. Wang, S. S. P. Parkin, B. A. Bernevig, and T. Neupert, Sci. Adv. **4**, eaat0346 (2018).
